# Supplementary material for: Shaping electron wave functions in a carbon nanotube with a parallel magnetic field
Source: arXiv:1712.08545 ancillary file (2019-03-07)
Supplement: Supplementary file 1 [file supplement.pdf]

# Shaping electron wave functions in a carbon nanotube with a parallel magnetic field
# Supplementary Material

Magdalena Marganska,[1] Daniel R. Schmid,[2] Alois Dirnaichner,[2] Peter L. Stiller,[2] Christoph Strunk,[2] Milena Grifoni,[1] and Andreas K. Hüttel[2]

[1]*Institute for Theoretical Physics, University of Regensburg, 93053 Regensburg, Germany*
[2]*Institute for Experimental and Applied Physics, University of Regensburg, 93053 Regensburg, Germany*

(Dated: February 22, 2019)

## CONTENTS

I. Device fabrication and measurement 1

II. Source vs. drain resonance 1

III. Modelling the CNT spectrum 2
A. Effective Hamiltonian 2
B. Orbital moment correction $\mu_x$ 3
C. On the nature of shells $\alpha$ and $\beta$ 4

IV. Transport calculation 6
A. Modelling the differential conductance 6
B. Suppression of the conductance with varying $\Gamma_{n\tau}$ 7

V. Soft confinement potential 8

VI. Low magnetic field measurements and minimal model 10

VII. Comparison with a perpendicular magnetic field 11

References 12

## I. DEVICE FABRICATION AND MEASUREMENT

On a highly p-doped silicon substrate with 300 nm thermal surface oxide, 40 nm thick rhenium contact electrodes were deposited via standard electron beam lithography, dc-sputtering and lift-off. Following anisotropic dry etching to deepen the trenches between the electrodes, in an additional lithography step growth catalyst was locally deposited close to the electrodes and CNTs were grown *in situ* via chemical vapour deposition.[1] After the growth, no further wet processing or imaging was performed to fully take advantage of the clean, as-grown macromolecules.[2,3]

Measurements were performed in an Oxford Instruments TLM dilution refrigerator with rotatable sample holder, at a base temperature of $\sim 30$ mK. The gate voltage was applied to the chip substrate, the bias voltage to a source contact; the resulting dc current at the corresponding drain contact was amplified and recorded. The magnetic field direction with respect to the nanotube was calibrated by recording transport spectra at varying angle and identifying the symmetry points.[4] The data was recorded using the Lab::Measurement software package.[5]

Since the contact with the rhenium leads is extended, the main bottleneck for tunneling occurs at the tunneling barrier between the electrostatically defined quantum dot and the rest of the nanotube. This contact dominates the transport characteristics of the device.

## II. SOURCE VS. DRAIN RESONANCE

In Figure 2(c) of the main text, the conductance resonances lowermost in bias voltage $V_{\text{bias}}$ abruptly change both curvature and amplitude in the magnetic field range $4\,\text{T} \lesssim B_{\|} \lesssim 8\,\text{T}$ (i.e., when reaching $V_{\text{bias}} = 0$). This behaviour can be explained by reminding us of the measurement technique. The conductance traces in Figures 2(b) and 2(c) are recorded at constant gate

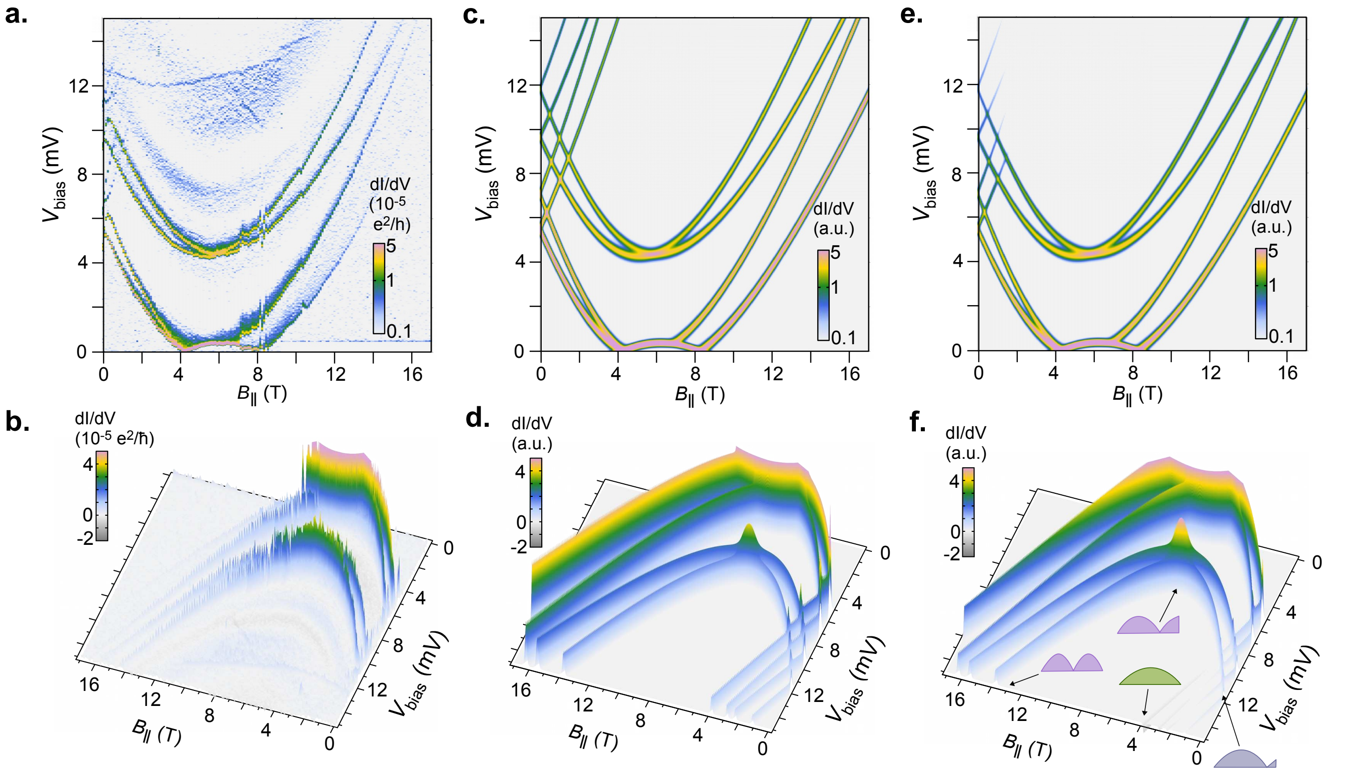


**Supplementary Figure S-1**. **Comparison of measurement data and modelling results with and without field-dependent tunneling rates (particle in a box vs. nanotube cross-quantization model). —** (a, b) Differential conductance at constant $V_{gate} = 0.675\,V$. Identical to Figs. 2(c) and 5(b) in the main text. (c, d) Calculated conductance, using the reduced density matrix technique and assuming field-independent tunneling coupling of all states to the leads. Identical to Fig. 2(d) in the main text. (e, f) Differential conductance calculated using the cross-quantization condition, Eq. (3), and thus field-dependent tunneling couplings. Identical to Fig. 5(a) of the main text.

voltage $V^*_{gate} = 0.675\,V$. As an example, the conductance trace $dI/dV_{bias}(B_\| = 0, V_{bias})$ from Figure 2(b) and Figure 2(c) is equivalent to the conductance trace $dI/dV_{bias}(V_{gate} = 0.675\,V, V_{bias})$ from the measurement of Figure 2(a).

Applying a magnetic field shifts the gate voltage position of the charge degeneracy point visible in Figure 2(a), where single electron tunneling is possible at zero bias. When increasing the magnetic field parallel to the carbon nanotube axis above $B_\| \simeq 4\,T$, this degeneracy point crosses the gate voltage value $V^*_{gate}$ chosen in Figures 2(b) and 2(c). Consequently, for the magnetic field range $4\,T \lesssim B_\| \lesssim 8\,T$ the constant gate voltage traces of Figure 2(c) at low bias do not cut through the $N = 0$ band gap region, but through the $N = 1$ charge occupation Coulomb blockade region instead. At the edge of the $0 \le N \le 1$ single electron tunneling region, visible in Figure 2(c) as the first line of finite differential conductance, the electrochemical potential of the quantum dot is for $4\,T \lesssim B_\| \lesssim 8\,T$ aligned with the Fermi edge of the *source* contact, not the *drain* contact as is the case outside this magnetic field range. Thus, a significantly stronger conductance signal is observed for this field range.

## III. MODELLING THE CNT SPECTRUM

### A. Effective Hamiltonian

As the basis for our calculation we use a standard tight-binding model of the CNT, taking into account all four valence electrons of the carbon atoms,[6,7] with three modifications. This effective Hamiltonian in the neighbourhood of the Dirac points is then given by

$$H_{CNT}(B_\|) = \sum_{m=0,1} \sum_{\tau,\sigma,\kappa_\|} \hbar v_F \left[\tau\kappa_\perp(B_\|)\, s_x + \kappa_\|(B_\|)\, s_y\right] + \tau\sigma\, \varepsilon_{SO} + \sigma\, \mu_B B_\| + \tau\mu_x B_\| + m\Delta_{\alpha\beta}, \tag{S-1}$$

where $\kappa_{\perp/\|}$ correspond to the momentum measured from the Dirac point in transverse and longitudinal directions, modified by the curvature effects and the spin-orbit coupling according to Eq. (1) of the main text. The Pauli matrices $s_x, s_y$ act in the

| parameter | $\alpha$ | $\beta$ |
|---|---|---|
| $\Delta k_{\perp}^{c}$ ($10^{-4}$/Å) | 10.5 | |
| $\Delta k_{SO}$ ($10^{-4}$/Å) | 0.05 | |
| $\varepsilon_{SO}$ (meV) | 0.25 | 0.35 |
| $\mu_x$ (meV/T) | -0.15 | -0.125 |
| $\Delta_{KK'}$ (meV) | 0.1 | 0.08 |
| $\Delta_{\alpha\beta}$ (meV) | 1.45 | |
| $R$ (nm) | 2.2 | |
| $L$ (nm) | 400 | |

**Supplementary Table S-I**. Numerical values of the parameters used in Eq. (S-1) in order to reproduce the experimental data.

sublattice space. The valley index is $\tau = \pm 1$ for the $K/K'$ valley, the spin index $\sigma = \pm 1$ for the spin projection onto the direction of the CNT axis. Spin-orbit coupling contributes to the Hamiltonian through two terms, $\Delta k_{SO}$ (orbital-like in the language of Ref. 8) and $\varepsilon_{SO}$ (Zeeman-like in the same terminology).

Our first modification consists of taking into account the dependence of $\kappa_{\parallel}$ on the magnetic field through the cross-quantization condition, Eq. (3) of the main text. The remaining two modifications are the last two terms of the Hamiltonian, Eq. (S-1), which reflect the particular nature of our device.

First, we are able to consistently fit the positions of the energy levels only by adding a constant contribution $\mu_x$ to the orbital magnetic moment corresponding to about 1/5 of the value of the orbital moment at zero field. A more detailed discussion of this can be found below in Section III B.

Second, the sets of states $\alpha$ and $\beta$ are very closely spaced in energy and very similar in their $B_{\parallel}$ dependence. An explanation for this – that our device may be a bundle of two CNTs (which occurs in our growth process and has been observed frequently in other processes as well)[9] with very similar chiralities – is discussed in detail in Section III C. In Eq. (S-1), we assume a constant spacing between $\alpha$ and $\beta$, setting the index $m$ to $m = 0$ for set $\alpha$ and to $m = 1$ for set $\beta$.

The numerical values of all parameters in Eq. (S-1) used in our calculation are listed in Table **S-I**. Together with the cross-quantization condition, Eq. (3) in the main text, they yield the field-dependent electronic wave functions and energy levels.

### B. Orbital moment correction $\mu_x$

The main factor influencing the magnitude of the electronic orbital moment is the radius of the examined CNT. The resulting estimate of the orbital moment of an electron in the conduction band at Fermi velocity $v_F$ in a CNT of radius $r$ is[10] $\mu = ev_F r/2$. When the size quantization resulting in a finite value of $\kappa_{\parallel}$ is taken into account, the orbital moment is reduced, which can be seen by analyzing Equation (S-1). The variation of energy levels in $B_{\parallel}$is dominated by the Aharonov-Bohm contribution to $\kappa_{\perp}$. Neglecting for the moment the weaker dependence of $\kappa_{\parallel}(B_{\parallel})$ and the $\tau\mu_x B_{\parallel}$ term, we obtain

$$\mu_{\text{orb}}(B_{\parallel}) \simeq \frac{\partial E}{\partial \kappa_{\perp}} \frac{\partial \kappa_{\perp}}{\partial B_{\parallel}} = \frac{ev_F r}{2} \frac{\kappa_{\perp}(B_{\parallel})}{\sqrt{\kappa_{\perp}(B_{\parallel})^2 + \kappa_{\parallel}^2}} \leq \frac{ev_F r}{2},$$

and therefore the estimate from the radius is also the upper limit on the value of $\mu_{\text{orb}}$. It is attained at high magnetic fields for which $\kappa_{\parallel} \ll \kappa_{\perp}(B_{\parallel})$. This can be seen also in Figure 1(d) of the main text, where the slope of $\partial E/\partial B_{\parallel}$ for all states approaches the classical limit only at large $B_{\parallel}$. The two main conclusions from this analysis are: (a) that the magnitude of the orbital moment at low fields is expected to be lower than that at the large fields, and (b) that the orbital moment is directly proportional to the nanotube radius $r$.

Figure **S-2**(a) shows the obviously poor fit of the energy levels to the conductance peak positions using the parameters given in Table **S-I**, but setting $\mu_x = 0$. Figure **S-2**(b) shows a comparison of $\mu_{\text{orb}}$ calculated from the theoretical fit (lines) and experimental data (points) for the four excitation lines attributed to the valley $K'$. The experimental derivatives were obtained by first fitting the peak positions with third order polynomials, then sampling their derivatives at discrete values of $B_{\parallel}$ and removing the appropriate Zeeman factor $\pm\mu_B$. Surprisingly, the experimental $\mu_{\text{orb}}$ has a higher absolute value at low than at high fields.

Unexpectedly high values of the orbital moment at low fields have already been reported several times,[11–15] which still consitutes a puzzle. The data presented in literature so far explored reliably only the regime of low magnetic fields, which is why the unexpectedly *low* value of $\mu_{\text{orb}}$ at *high* fields observed in our work was not noticed before. Independent of the physical origin of this modification of orbital magnetic moment, it seems to be captured by the phenomenological term $\tau\mu_x B_{\parallel}$ added to

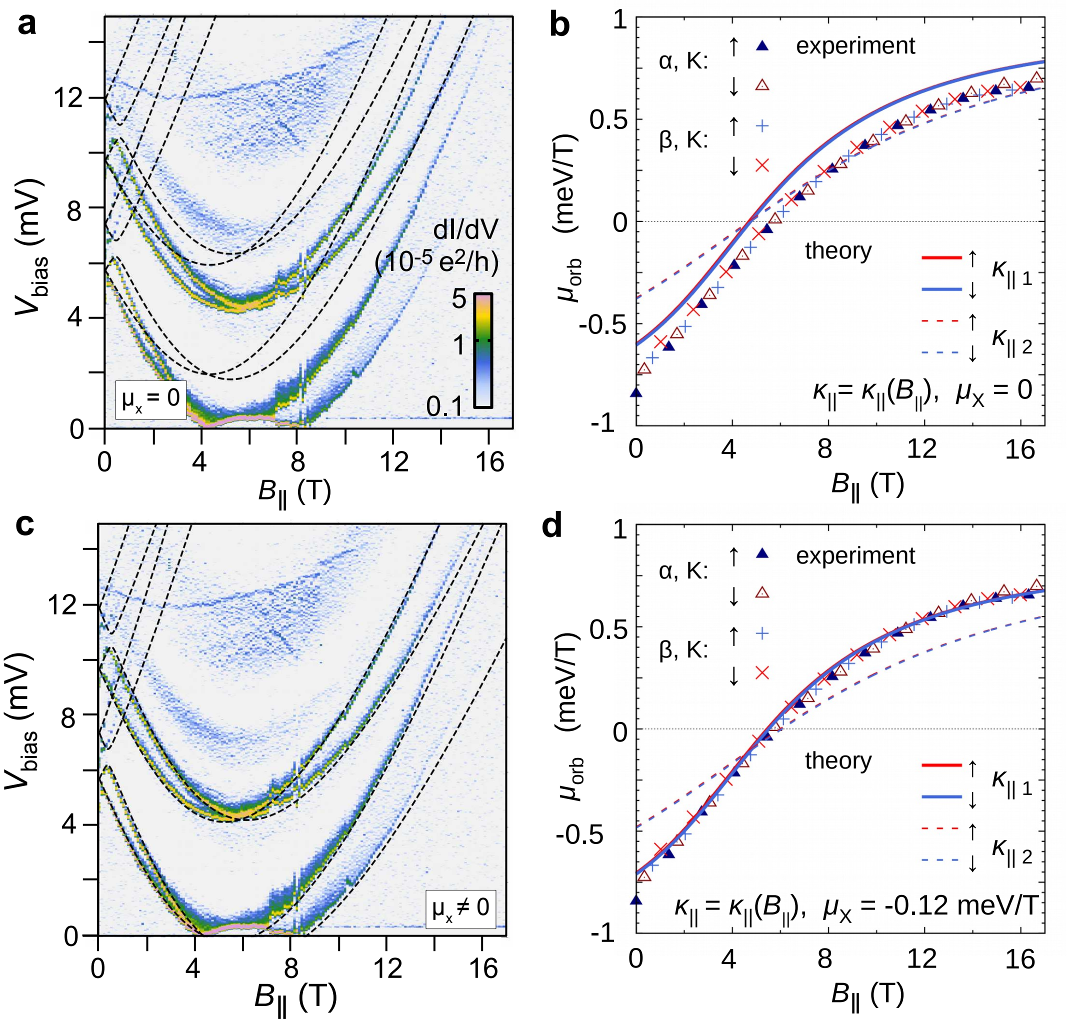


**Supplementary Figure S-2**. **Excitation spectrum and orbital moments. —** (a) Color plot of the differential conductance (cf. Figure 2(c) of the main text) and theoretically calculated position of the conductance peaks (dashed lines) when no $\mu_x$ correction to the CNT Hamiltonian (see Equation (S-1)) is included. (b) The orbital magnetic moment $\mu_{\mathrm{orb}} = \partial E / \partial B_{\|}$ for the four $K'$ excitation lines in shells $\alpha$ and $\beta$. Points correspond to the orbital moments obtained from the experimental data, continuous lines to the theoretical lines associated to wave functions $\psi_{1K'}(x_{\|}, B_{\|})$. Note that all four experimental lines display nearly the same evolution with $B_{\|}$, similar to the $\kappa_{\|1}$ theoretical line describing the lowermost longitudinal momentum, while the theoretical line with $\kappa_{\|2}$ has a clearly different shape. (c) Differential conductance and theoretical calculation of $dI/dV_{\mathrm{bias}}$ peak positions, now including the $\mu_x$ term. (d) The same plot as in (b), with the theoretical lines shifted by a constant $\mu_X = -0.12\,\mathrm{meV}$. A good agreement of all experimental data with the $\kappa_{\|1}$ theoretical line is found, strongly indicating that both shells $\alpha$ and $\beta$ correspond to the same longitudinal ground state wave function.

the Hamiltonian as in Equation (S-1). The conductance peak positions with this term included agree with the experimental data remarkably well, as shown in Figure S-2(c) and in Figure S-2(d) for the magnetic moment.

### C. On the nature of shells $\alpha$ and $\beta$

The remarkable similarity in the magnetic field evolution of all experimental orbital moments in Figure S-2(b,d) is at odds with the assumption that the shells $\alpha$ and $\beta$ belong to different longitudinal modes, i.e., different quantized values of $\kappa_{\|}$. The theoretical calculation of the orbital moment for $\kappa_{\|1}$ and $\kappa_{\|2}$ is shown in Figure S-2(b,d) with solid and dashed lines, respectively. The shell $\beta$ should evolve along the dashed line corresponding to $\kappa_{\|2}$, but shows instead a stronger dependence on the magnetic field, consistent with the same $\kappa_{\|1}$ as the shell $\alpha$.

Moreover, a curious feature of the transport spectrum in Figure 2(a) of the main text is the absence of higher excited states

above the quadruplet $\beta$. For the cross-quantization model described in the main text, as well as for a simple box potential or a harmonic confinement, regularly spaced energy levels corresponding to the longitudinal wavefunction quantization should emerge.

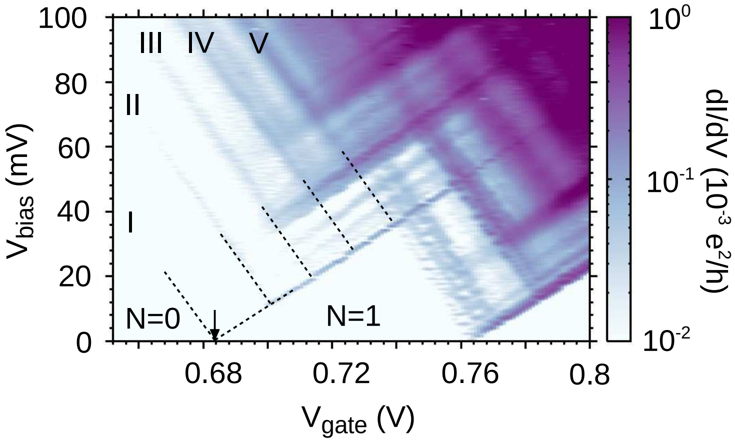


**Supplementary Figure S-3**. **Higher shell excitations. —** Differential conductance $\mathrm{d}I/\mathrm{d}V_{\mathrm{bias}}(V_{\mathrm{gate}}, V_{\mathrm{bias}})$ measured close to the band gap of the nanotube device, with dc bias voltages up to 100 mV and zero magnetic field. A regular pattern of excitations emerges as differential conductance lines. The energy spacing between these large scale excitations is on the order of 8 meV. We interpret them as consecutive longitudinal momentum shells, numbering them as I to V. Figure 2(a) of the main text is a high resolution detail measurement of the region between $N = 0$ and $N = 1$ dot occupation, i.e., close to the position marked here with a black arrow.

Indeed an overview measurement of the $N = 0$ to $N = 1$ region, shown in Figure S-3, displays a distinct, repetitive energy spacing between excitations of $\Delta E \sim 8\,\mathrm{meV}$, much larger than the spacing between shells $\alpha$ and $\beta$. We can attribute this energy scale $\Delta E$ to discrete longitudinal momentum states due to the finite size quantization in a nanotube quantum dot with $L \simeq h v_F \pi/\Delta E \sim 240\,\mathrm{nm}$.[16] This again poses the question of the nature of $\alpha$ and $\beta$, with a much smaller intershell spacing of $\Delta_{\alpha\beta} = 1.45\,\mathrm{meV}$. Their presence hints at an additional degeneracy associated with an additional degree of freedom in the system.

There may be several sources of such a degeneracy; generally, they fall into two broad categories, which may be viewed as "doubling in series" and "doubling in parallel". An example of the former category of "doubling in series" is the formation of a low tunnel barrier (e.g., due to an impurity) at the center of the nanotube, resulting in the creation of a strongly coupled double quantum dot. Each of the constituent dots would then host the usual quadruplet of states, and the experiment would record excitation lines corresponding to their bonding and antibonding combinations. We have considered this scenario and rejected it for two reasons. First, both the detuning $\Delta$ between the energy levels of each dot and the tunnel splitting between them $2t_0$ would have to be smaller than the observed intershell spacing $\Delta_{\alpha\beta}$. Using the rough estimate of the energy quantization in the dot, $\Delta E \approx \hbar v_F \pi/L$, and for $\Delta \lesssim \Delta_{\alpha\beta}/2$, the difference between the lengths of the left and right dot would have to be smaller than 50 nm. Though statistically unlikely, this might yet occur in our device. Second, we have performed numerical tight-binding simulations of carbon nanotubes with central tunneling barriers of various heights and shapes. The calculations show that the stronger hybridization between the left and right parts of the CNT leads to a decrease in the orbital magnetic moment at low fields, which in our device is strongly enhanced instead.

The second category of "doubling in parallel" assumes the presence of two weakly coupled nanotubes running parallel for at least a part of their length, i.e. forming a bundle or a Y junction. The hybridization would then occur along the part where the two CNTs are joined. The coupling must be strong enough that the two CNTs do not register as separate quantum dots, since the stability diagram shows only one pattern of Coulomb oscillations. We have tested this hypothesis by real space numerical tight-binding calculations of the spinless electron spectra for several bundles consisting of two CNTs. The nanotubes were assumed to be straight and parallel to each other along their whole length. The intertube coupling was modelled as a weak tunneling hopping between atoms belonging to the different bundle members, with the tunneling amplitude decaying exponentially with the distance between the hopping sites. This model has been used elsewhere to account for the coupling between the outer and inner wall of a double-wall nanotube.[17–19] The resulting electronic spectra of four two-nanotube bundles with different chiralities are shown in Figure S-4. In the case of two identical constituent nanotubes, Figure S-4(a) or Figure S-4(b), the quadruplets of states at lowermost longitudinal momentum hybridize into an octuplet, forming two energetically close shells similar to our measurement. When combining two nanotubes of different chirality, Figure S-4(c) or Figure S-4(d), we obtain an octuplet of states in two differing groups. In both cases, the inter-tube hybridization and the breaking of rotational symmetry leads to valley mixing, i.e., a finite $\Delta_{KK'}$ term causing broken degeneracy at zero magnetic field.

## IV. TRANSPORT CALCULATION

### A. Modelling the differential conductance

The amplitudes of the wave functions at the nanotube ends were used to determine the field and valley-dependent tunneling couplings to the leads, $\Gamma_{l\mu}(B_{\|})$. In order to calculate the transport through the quantum dot we set up a generalized master equation for the reduced density matrix,[20] in a sequential tunneling regime. In the range of gate and bias voltages shown in the main text only states with $N=0$ and $N=1$ are populated. Since tunneling through $N>1$ states can be neglected, the rate equations for the stationary density matrix $\rho$ acquire a simple form,

$$0=\sum_{l}\Gamma^{+}_{l\mu}\rho_0-\sum_{l}\Gamma^{-}_{l\mu}\rho_\mu, \tag{S-2}$$

$$0=-\sum_{l,\mu}\Gamma^{+}_{l\mu}\rho_0+\sum_{l,\mu}\Gamma^{-}_{l\mu}\rho_\mu, \tag{S-3}$$

where $\rho_0$ is the population of the $N=0$ state and $\rho_\mu$ are populations of the $N=1$ states, each with the collective quantum number $\mu=\{n,\tau,\sigma\}$. The index $l=L,R$ denotes the left or right lead, respectively. The rates $\Gamma^{\pm}_{l\mu}$ are the rates for tunneling into $(+)$ or out of $(-)$ the state $\mu$ through the lead $l$ and are given by

$$\Gamma^{\pm}_{l\mu}=\frac{2\pi}{\hbar}\alpha_l|\psi_\mu(x=x_l,B_{\|})|^2 f^{\pm}_l(\varepsilon_\mu), \tag{S-4}$$

with

$$f^{+}_l(\varepsilon)=\left[1+\exp\left(\frac{\varepsilon-\mu_l}{k_BT}\right)\right]^{-1},\quad f^{-}_l(\varepsilon)=1-f^{+}_l(\varepsilon) \tag{S-5}$$

the Fermi-Dirac functions of the leads with their corresponding chemical potentials $\mu_l=\varepsilon_{F,l}-eV_l$, where $\varepsilon_{F,l}$ is the initial Fermi level of the lead $l$ and $V_l$ the applied voltage. The rates in Eq. (S-4) depend on the magnetic field in two ways. First, through the dot single particle energy $\varepsilon_\mu$ and second, through the amplitude of the wave functions of states $\mu$ at the contacts, which we take to be symmetric and dependent on the magnetic field. In our case there are eight single particle states to be occupied, with $\tau=\pm1,\sigma=\pm1$ and $n=1$ in the $\alpha$ or $\beta$ shell. The factors $\alpha_l$ contain the density of the lead states at the contact and encode possible asymmetry between the coupling of the quantum dot to the left and right lead. The equations above are not linearly

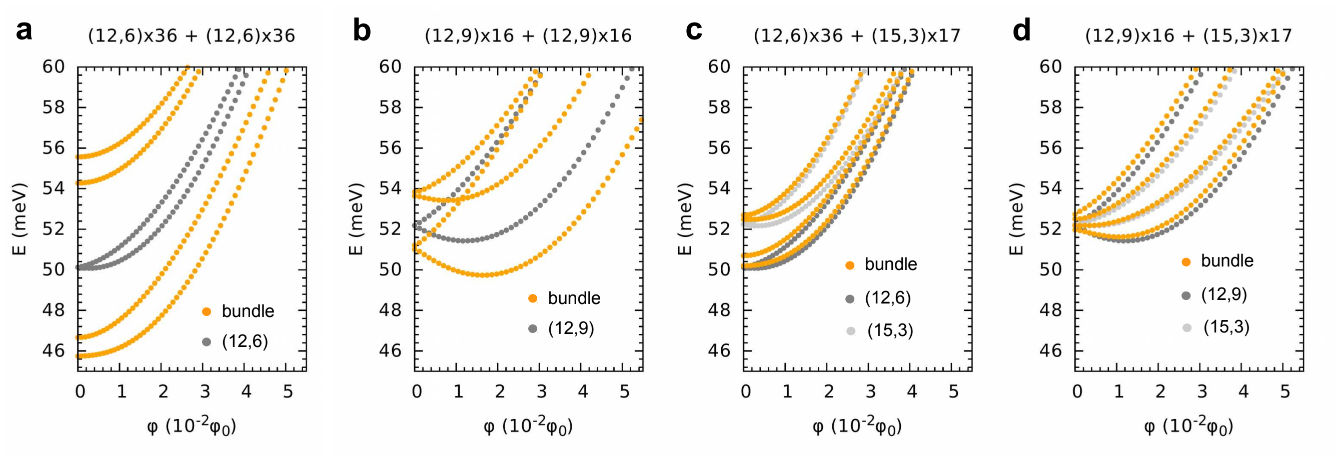


**Supplementary Figure S-4**. **Spectra of carbon nanotube bundles.** — Spinless electron spectra of two-nanotube bundles with different chiralities, obtained via numerical tight binding calculations and assuming a hybridization of quantum states along the entire bundle length. Orange points correspond to the spectra of a bundle with included intertube tunneling, the light and dark grey points to the energy levels of the two individual nanotubes in the bundle. (a,b) In bundles of (12,6)+(12,6) and (12,9)+(12,9) nanotubes, i.e., equal chirality, the individual nanotube states are strongly hybridized by the tunneling. (c,d) In bundles consisting of two different nanotubes, here (12,6)+(15,3) and (12,9)+(15,3), the tunneling manifests through a small shift of individual spectral lines and a valley mixing caused by the breaking of rotational symmetry, visible in the removal of level degeneracy at $B_{\|}=0$.

independent, and one of them can be replaced, e.g., by the normalization condition $\sum_\mu \rho_\mu + \rho_0 = 1$. We solve them numerically and calculate the resulting current in the stationary limit as

$$I_l = e\sum_\mu \Gamma^+_{l\mu}\rho_0 - \sum_\mu \Gamma^-_{l\mu}\rho_\mu .$$

The derivative of this current with respect to the bias voltage yields the differential conductance.

The steady *decrease* of $\Gamma_{l1K\sigma}$ with magnetic field suppresses the $K$ excitation lines, at some point turning them into blocking states with the associated negative differential conductance (NDC), faintly visible in Fig. 5(a) though in the experimental data they are drowned by a noisy background. We discuss those NDC features in more detail in Section IV B below, using a minimal model which neglects the shell and spin degrees of freedom and keeps only the valley, together with its wave functions tunable with the magnetic field.

Numerical calculations were performed using the Armadillo library.[21]

### B. Suppression of the conductance with varying $\Gamma_{n\tau}$

As already mentioned, the transport through the weakly coupled $K$ states at low magnetic fields can become suppressed to the point where even negative differential conductance features appear. Our CNT quantum dot hosts eight single-particle states, but such a suppression of transport would occur even within a minimal system containing only one $K$ and one $K'$ state. In the following we shall discuss such a minimal two-state setup, denoting the lower / higher energy state of an $N = 1$ quantum dot by $K'$ / $K$, respectively. The coupled equations for the stationary reduced density matrix, in the regime of sequential tunneling between $N = 0$ and $N = 1$ quantum dot states, are

$$-\sum_{l\tau}\Gamma^+_{l\tau}\rho_0 + \sum_{l\tau}\Gamma^-_{l\tau}\rho_\tau = 0, \qquad \sum_l \Gamma^+_{l\tau}\rho_0 - \sum_l \Gamma^-_{l\tau}\rho_\tau = 0, \tag{S-6}$$

where $\rho_0$ denotes the population of the $N = 0$ state and $\rho_{K/K'}$ the population of the respective single particle states. The rates $\Gamma^+_{l\tau}$ describe the tunneling into $(+)$ or out of $(-)$ the state $\tau$ through the lead $l$. They are given by a product of Eq. (4) from the main text and the appropriate Fermi-Dirac functions,

$$\Gamma^\pm_{l\tau} = \frac{2\pi}{\hbar}\alpha_l |\psi_\tau(x = x_l, B_\parallel)|^2 f^\pm_l(\varepsilon_\tau), \tag{S-7}$$

For simplicity we shall use in the following the abbreviation $|\psi_\tau| := |\psi_\tau(x = x_R, B_\parallel)| = |\psi_\tau(x = x_L, B_\parallel)|$. The rate equations, completed with the normalization requirement $\rho_0 + \sum_\tau \rho_\tau = 1$, are then solved numerically, and the current calculated. The current in the lead $l$ is given by the rates at which the dot states are populated and depopulated through this lead,

$$I_l = e\sum_\tau (\Gamma^+_{l\tau}\rho_0 - \Gamma^-_{l\tau}\rho_\tau). \tag{S-8}$$

In the experimental setup the bias is applied only to the left lead, with the right lead grounded. This makes the differential conductance $dI_R/dV_{\text{bias}}$ particularly easy to calculate, since the rates $\Gamma^\pm_{R\tau}$ do not depend on the bias. We have thus

$$\frac{dI_R}{dV_{\text{bias}}} = (\Gamma^+_{RK} + \Gamma^+_{RK'})\frac{d\rho_0}{dV_{\text{bias}}} - \Gamma^-_{RK}\frac{d\rho_K}{dV_{\text{bias}}} - \Gamma^-_{RK'}\frac{d\rho_{K'}}{dV_{\text{bias}}}. \tag{S-9}$$

Inserting equation (S-7) and populations calculated from Equation (S-6) into (S-9), we obtain

$$\left.\frac{dI_R}{dV_{\text{bias}}}\right|_{eV_{\text{bias}}=\varepsilon_K} = \frac{e}{k_B T}\frac{\alpha_L\alpha_R^2(\alpha_L+\alpha_R)}{[(\alpha_L+2\alpha_R)^2 - 2\alpha_R^2]}\left(-(\alpha_L+\alpha_R)|\psi_K| + \alpha_L|\psi_{K'}|\right). \tag{S-10}$$

When the magnetic field grows beyond $B_0$, defined as such that the wave function amplitudes $|\psi_\tau(B_0)|$ fulfill

$$\frac{|\psi_K(B_0)|^2}{|\psi_{K'}(B_0)|^2} = \frac{\alpha_L}{\alpha_L+\alpha_R}, \tag{S-11}$$

the conductance at $eV_{\text{bias}} = \varepsilon_K$ becomes negative. The population of the well coupled state $K'$ becomes depleted in favour of the weakly coupled state $K$. For magnetic fields $B_\parallel > B_0$ the opening of another channel does not compensate anymore the drop in the population of the $K'$ state and the overall current decreases.

Figure **S-5** shows the differential conductance of a quantum dot with two spinless $K$ and $K'$ states whose energy levels evolve in the magnetic field like those shown in Figure 1(d) of the main text. The left panel in Figure **S-5** plots the $dI_R/dV_{\text{bias}}$ calculated

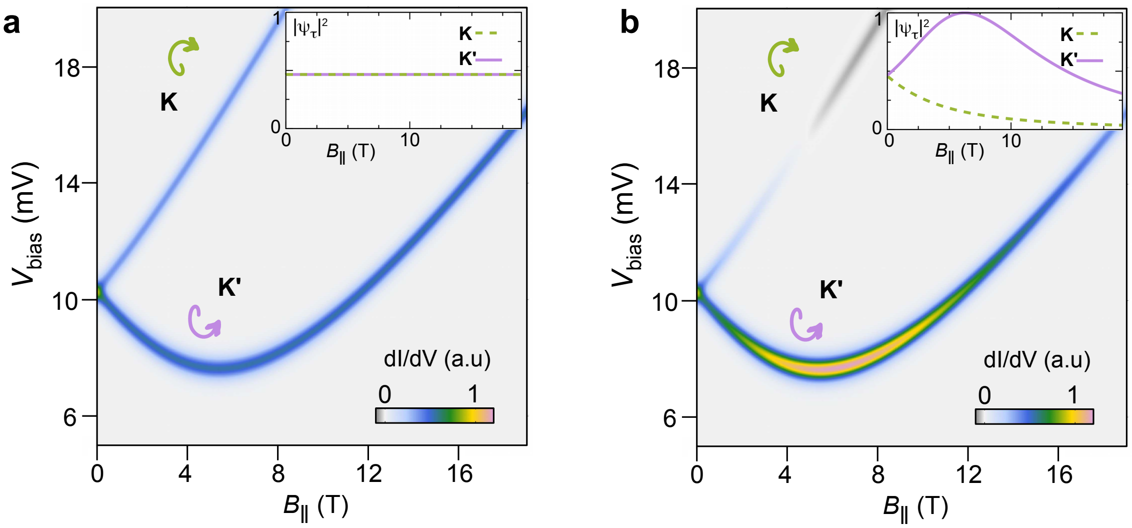


**Supplementary Figure S-5. Transport through a CNT quantum dot with two levels.** — Differential conductance calculated from Eq. (S-9) for a CNT quantum dot, with (a) constant and (b) magnetic-field dependent amplitudes for $\psi_{K'}$ and $\psi_K$ at the contacts. The insets show the values of $|\psi_\tau|^2$ at the contacts as functions of the magnetic field. The dependence of $|\psi_\tau|$ on the magnetic field is the same as that of $|\psi_{1\tau}|$ which yielded the results shown in Fig. 5 of the main text.

with the assumption of $|\psi_\tau| = \text{const} = |\psi_\tau(B_\| = 0)|$, while the right panel shows $dI_R/dV_{\text{bias}}$ for field-dependent $|\psi_\tau|$. In both calculations $\alpha_L/\alpha_R = 1/4$, as in the main text; the temperature is set to $T = 1.5$ K in order to broaden the excitation lines, enhancing their visibility. The conductance of the $K$ and $K'$ lines in Figure S-5(a) remains nearly constant across the magnetic field, while in Figure S-5(b) the $K'$ lines clearly gain initially in strength, while the $K$ lines fade out, their differential conductance turning negative beyond $B_\| \simeq 5$ T, according to our expectations.

## V. SOFT CONFINEMENT POTENTIAL

In the main text we have studied the evolution of electronic wave functions assuming an atomically sharp termination of the CNT quantum dot. To answer the question whether a similar effect would persist if the quantum dot was defined by a soft, electrostatic confinement potential, we have performed numerical calculations of the transmission through a smoothly confined quantum dot, using Green's functions techniques. The local density of states at each atom corresponds to the squared local amplitude of the wave function in a closed system. The nanotube we chose for illustration is the same as in the main text, i.e. a (15,3) CNT.

Figure S-6(a) shows a schematic of a sharply confined quantum dot weakly connected to the leads by the atoms at its boundary. The grey regions represent the contacts. We shall examine closely the lowest $K/K'$ pair of extended eigenstates, corresponding to $\psi_{1K}$ and $\psi_{1K'}$ in Figure 4 of the main text. The evolution of the amplitude at the contacts, the acquisition of another node by the wavefunction of the $K'$ states and the loss of one antinode by the wave function of the $K$ states are clearly visible. Note also that, as a side effect of the wave functions tending asymptotically to the half-wave shape, their profiles, different on the $A$ and $B$ sublattice at $\phi \approx 0$, overlap almost completely at $\phi = 0.08\phi_0$.

For the device with soft-confined quantum dot we chose as the central part a nanotube with 100 unit cells, corresponding to a length of 237.3 nm, with the dot formed in the potential well in its center. The soft confinement was imposed through an on-site potential term given by

$$V(x_\|) = \frac{V_0}{2}\left(2 - \tanh\left(\frac{x_\| - x_L}{\Delta x_L}\right) + \tanh\left(\frac{x_\| - x_R}{\Delta x_R}\right)\right),$$

which yields a potential well with the bottom at $V(x_\|) = 0$ and with height $V_0$ at the left and right end. The parameters $x_{L/R}$ set the position of the left and right well walls respectively and $\Delta x_{L/R}$ the softness of the potential. In Figure S-6(b) we used $x_L = 0$ nm, $x_R = 137.6$ nm, $\Delta x_L = \Delta x_R = 8$ nm and $V_0 = 40$ meV. The resulting shape of the potential well is shown in Figure S-6(b) as the grey filled curves. The leads are simulated as semi-infinite p-doped CNTs, which was achieved by setting their electrostatic potential to be level with the top of the well. The p-doping of the leads in the experiment is inferred from the gate traces shown

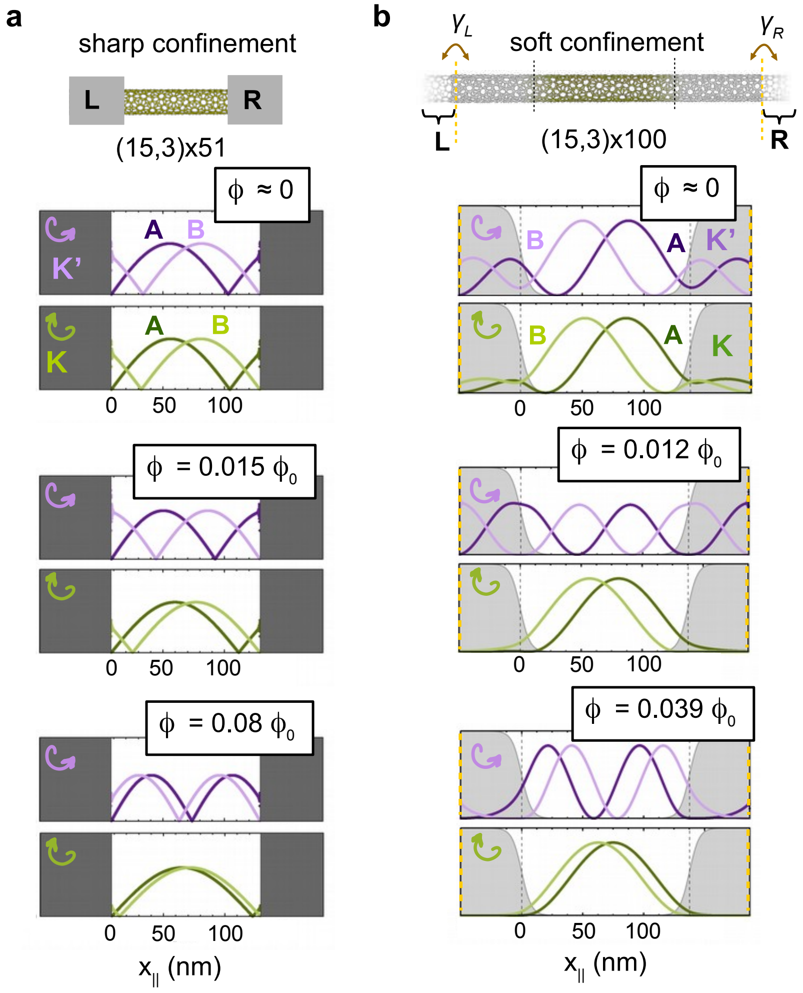


**Supplementary Figure S-6**. **Sharp vs. soft confinement.** — (a) The shape of $K'$ and $K$ wave function amplitudes $|\psi_{1\tau}(B_\parallel, x_\parallel)|$ for the longitudinal mode with $n=1$ at three values of magnetic flux. These are similar to the shapes shown in Figure 4 of the main text, for a device with sharp nanotube ends weakly connected to the leads. The CNT has the chirality (15,3) with 51 unit cells. Its length is 121 nm. At the highest value of the magnetic flux the wave functions on the two sublattices become markedly similar. (b) The local density of states (LDOS) in a quantum dot of similar length as in (a), but created by imposing a smoothly varying electrostatic potential on an infinite nanotube. The semi-infinite segments beyond the orange lines are CNT leads, with a nearly transparent tunneling interface to the central part, $\gamma_L = \gamma_R = 0.8V_\pi$. The quantum dot is located in the potential well formed in the central part of the nanotube. $x_\parallel = 0$ is set to coincide with the center of the left slope of the potential well. As in the case of sharp ends, the amplitude of the $K'$ wave function at the interface between the quantum dot and the rest of the nanotube initially increases, enhancing the transmission through the $K'$ state. The amplitude of the $K$ state at the (now extended) interface steadily decreases with increasing magnetic flux.

in Fig. S-10, where $V_{\text{gate}} = 0$ is in the valence band. The hopping from the leads (CNT segments lying on rhenium) to the central (suspended) part is only slightly smaller than the lattice hopping, $\gamma_L = \gamma_R = 0.8V_\pi$.

The evolution of the wave functions in a soft-confined dot, here given by their local density of states (LDOS), shows similar characteristics as for the sharply terminated dot. Their amplitudes at the contacts also have an initial increase for the $K'$ state followed by a decrease, while the amplitude of the $K$ state is suppressed from the beginning.

The p-n junction regions (the "walls" of our potential well) set the boundary conditions for the amplitude of the LDOS outside the quantum dot. Accordingly, a suppression of the LDOS amplitude at the slope of the potential well and subsequently in the shaded region of Fig. S-6(b) corresponds to lower conductance through the specific quantum dot state. For example, the state $K'$ at $\phi = 0.012\phi_0$ has an exceptionally good contact with the corresponding electronic state from the valence band in the leads – in fact, the LDOS seems almost unperturbed by the presence of the potential well. This good connection is caused by the high amplitude of the $K'$ state's wave function at the effective ends of the quantum dot $x_L, x_R$ - as we can see, the $K$ state at the same $\phi$ is nearly decoupled from the leads.

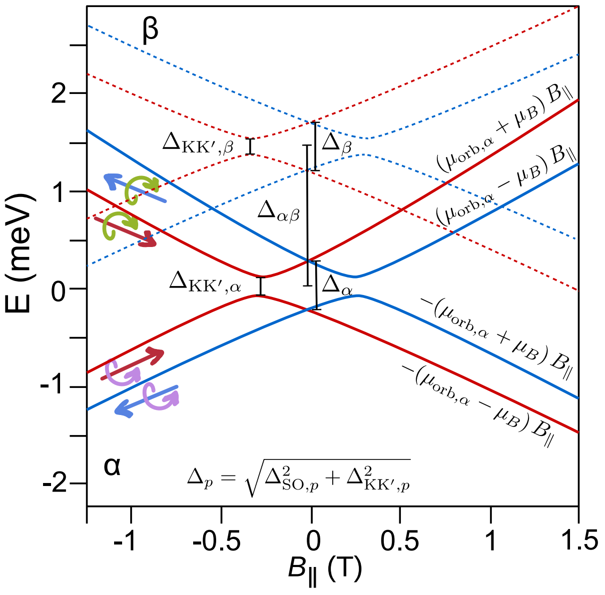


**Supplementary Figure S-7**. **Low field schematics of the energy levels. —** Schematics of the energy levels as present in the minimal model, with the quantities denoted as used in Equation (S-12).

The reshaping of the quantum dot wave function with the magnetic fields also still occurs, as is manifest in the fact that in each state at high field the nodal structure of the $A$ and $B$ sublattice components is nearly the same, see bottom panels of Figure **S-6**.

This analysis shows that while the shape of the confining potential certainly matters, the nature of the evolving dot wave functions is equally important for understanding the transport behaviour in high magnetic fields.

## VI. LOW MAGNETIC FIELD MEASUREMENTS AND MINIMAL MODEL

The spectrum of a carbon anotube at low parallel magnetic fields is determined predominantly by the linear response terms. It can be well reproduced by a minimal model[11,13,22] which, when adapted to our set-up, is given by the Hamiltonian

$$H_{CNT}(B_\parallel) = \sum_{m=0,1} m\Delta_{\alpha\beta}\, t_0 \otimes s_0 + \frac{\Delta_{SO,m}}{2}\, t_z \otimes s_z + \frac{\Delta_{KK',m}}{2}\, t_x \otimes s_0 + \frac{1}{2} g_s \mu_B B_\parallel\, t_0 \otimes s_z + \mu_{orb}\, B_\parallel t_z \otimes s_0, \tag{S-12}$$

where $t_i$ and $s_i$ are Pauli matrices acting in the valley and spin space, respectively. The constant $\Delta_{SO,m}$ is the spin-orbit splitting, $\Delta_{KK',m}$ the valley mixing and $\mu_{orb}$ the orbital moment in the shell $m$. These parameters, with the resulting spectrum, are illustrated schematically in Figure **S-7**. Figure **S-8** shows detail measurements at low magnetic field; the numerical values for the parameters of Equation (S-12) from fitting the data are given in Table **S-II**.

| parameter | $\alpha$ | $\beta$ |
|---|---|---|
| $\Delta_{SO}$ (meV) | 0.48 | |
| $\Delta_{KK'}$ (meV) | 0.2 | 0.15 |
| $\mu_{orb}$ (meV/T) | 0.82 | |
| $\Delta_{\alpha\beta}$ (meV) | 1.4 | |

**Supplementary Table S-II**. **Parameters for the minimal model Hamiltonian.** Numerical values of the parameters used in Equation (S-12) to reproduce the low-field experimental data.

The value of the orbital moment $\mu_{orb}$ automatically contains the contribution of $\mu_x$. However, we note a discrepancy, visible in Figure **S-8**(a). The experimental data seem to be tilted with respect to the theoretical lines; when this tilt is added to the minimal model, Eq. (S-12), as an overall $a_x B_\parallel$ term, $H_{CNT} \to H_{CNT} + a_x B_\parallel$, the theoretical lines follow the positions of experimental conductance peaks much closer, see Figure **S-8**(b-d).

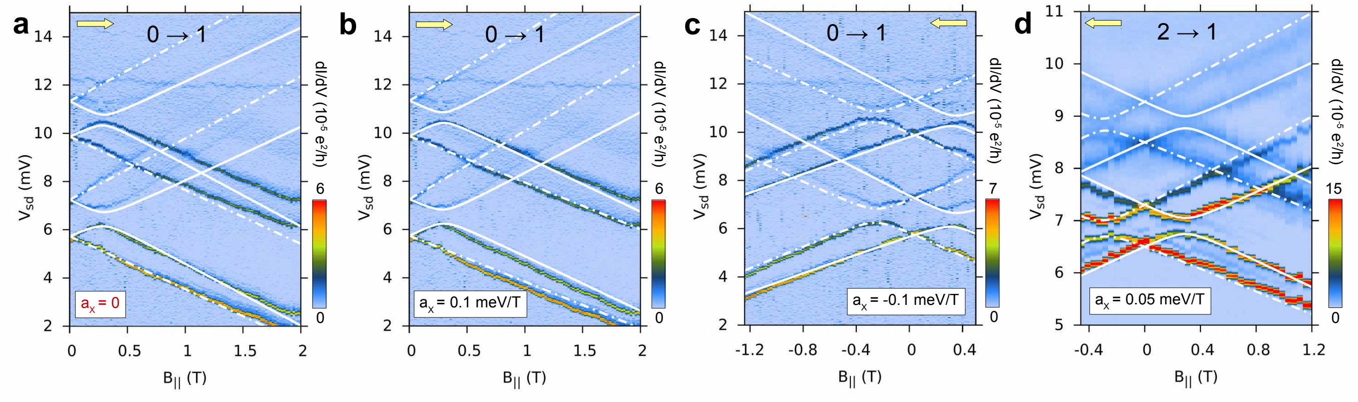


**Supplementary Figure S-8. Low magnetic field $B_{||}$ excitation spectra with fits from minimal model. —** (a,b) Differential conductance plot of the excitation lines as already shown in Figure 2(b) of the main text, with theoretical fits to the minimal model. The yellow arrow indicates the direction in which the magnetic field was varied in the experiment. Continuous lines mark the spin ↓ states, dot-dashed lines the spin ↑ states. In (a) the fit does not include the overall tilt $a_x$, in (b) it does (see text). (c) An additional measurement of the same region of the stability diagram. (d) Analogous measurement of the one-electron excitations as they become visible within the $1 \lesssim N \lesssim 2$ single electron tunneling region; $V_{\mathrm{gate}} = 0.77$ V. Here the conductance lines correspond to resonances with the *source* contact Fermi level.

The nature of the $a_x$ tilt is not clear. As visible from Figure S-8(b-d), measurements which should be fully equivalent lead to different values of the tilt parameter $a_x$. In particular because of the apparent dependence of the sign of $a_x$ on the stepping direction of the magnet power supply, we tentatively ascribe the need for this correction term to a so far unidentified systematical error in our magnetic field at the nanotube site. A similar overall tilt of the whole spectrum has already been reported, though also not understood.[23]

## VII. COMPARISON WITH A PERPENDICULAR MAGNETIC FIELD

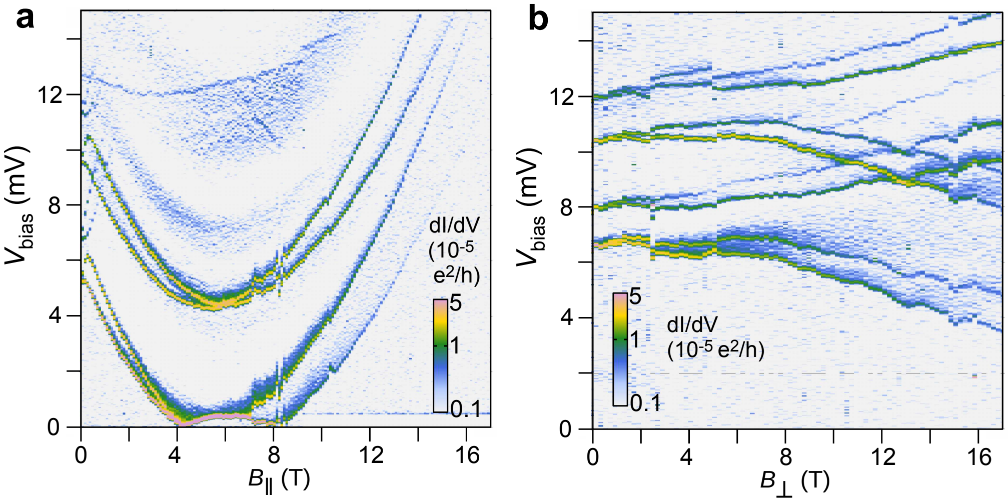


**Supplementary Figure S-9. Comparison of the effects of a parallel and a perpendicular magnetic field - excitation spectrum. —** (a) Excitation lines in a high parallel field, as shown in Fig. 2(c) of the main text. (b) The corresponding measurement in a field perpendicular to the nanotube axis registers all eight excitation lines. Their strength does vary, but much less than in the parallel field.

Since the variation of the longitudinal profile of the wave function described in this article is caused by the presence of an Aharonov-Bohm flux, we expect to see no modulation of conductance in a magnetic field perpendicular to the carbon nanotube axis, because such a field couples only to the spin, not to the valley. The variation in the position of energy levels is so small that

a minimal model similar to (S-12) holds even at high fields,

$$H_{\mathrm{CNT}}(B_\perp) = \sum_{m=0,1} m\Delta_{\alpha\beta}\, t_0 \otimes s_0 + \frac{\Delta_{\mathrm{SO},m}}{2}\, t_z \otimes s_z + \frac{\Delta_{\mathrm{KK}',m}}{2}\, t_x \otimes s_0 + \frac{1}{2} g_s \mu_B B_\perp\, t_0 \otimes s_x. \tag{S-13}$$

The comparison between the excitation lines in a parallel and in a perpendicular field, shown in Figure S-9, confirms our expectation. In the perpendicular field the strength of the excitation lines changes only weakly and all eight lines are present even at high field.

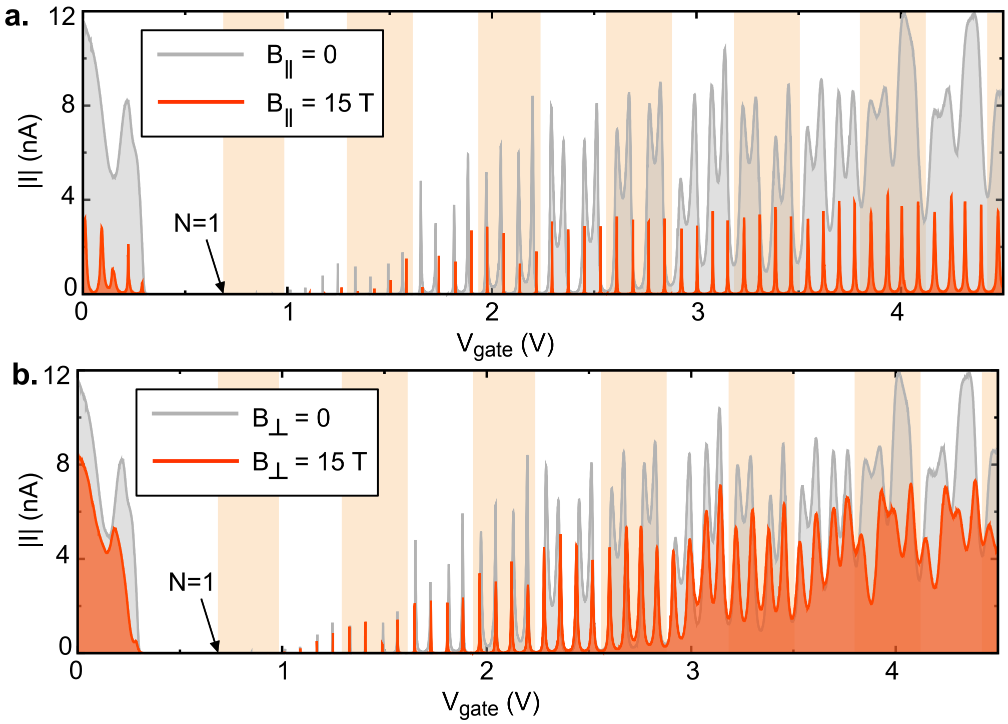


**Supplementary Figure S-10**. **Comparison of the effects of a parallel and a perpendicular magnetic field - zero bias trace. —** (a) Low bias ($V_{\mathrm{bias}} = -0.05\,\mathrm{mV}$) current measured at zero magnetic field and at a high parallel magnetic field $B_\| = 15\,\mathrm{T}$. The suppression of transport is so strong that at high field the quantum dot shows Coulomb blockade over nearly the whole gate voltage range. (b) The corresponding measurement in a field perpendicular to the nanotube axis shows only a weak suppression of the current.

We have also measured the low bias current at high parallel as well as perpendicular magnetic fields, under otherwise identical conditions, with the results shown in Figure S-10. As expected, the conductance is only weakly suppressed by the perpendicular field; the remaining suppression may be due to, e.g., a splitting of broad zero-bias Kondo conductance anomalies via the Zeeman effect. In a field parallel to the carbon nanotube axis, however, the suppression is so strong that it drives the device into the Coulomb blockade regime even at the highest electron number occupation depicted.


[1] J. Kong, H. T. Soh, A. M. Cassell, C. F. Quate, and H. Dai, "Synthesis of individual single-walled carbon nanotubes on patterned silicon wafers," Nature **395**, 878 (1998).

[2] J. Cao, Q. Wang, and H. Dai, "Electron transport in very clean, as-grown suspended carbon nanotubes," Nature Materials **4**, 745 (2005).

[3] A. K. Hüttel, G. A. Steele, B. Witkamp, M. Poot, L. P. Kouwenhoven, and H. S. J. van der Zant, "Carbon nanotubes as ultra-high quality factor mechanical resonators," Nano Letters **9**, 2547–2552 (2009).

[4] D. R. Schmid, S. Smirnov, M. Marganska, A. Dirnaichner, P. L. Stiller, M. Grifoni, A. K. Hüttel, and C. Strunk, "Broken SU(4) symmetry in a Kondo-correlated carbon nanotube," Phys. Rev. B **91**, 155435 (2015).

[5] S. Reinhardt, C. Butschkow, S. Geissler, A. Dirnaichner, F. Olbrich, C. Lane, D. Schröer, and A. K. Hüttel, "Lab::Measurement — a portable and extensible framework for controlling lab equipment and conducting measurements," Computer Physics Communications **234**, 216 (2019).

[6] W. Izumida, K. Sato, and R. Saito, "Spin-orbit interaction in single wall carbon nanotubes: Symmetry adapted tight-binding calculation and effective model analysis," Journal of the Physical Society of Japan **78**, 074707 (2009).

[7] J. Klinovaja, M. J. Schmidt, B. Braunecker, and D. Loss, "Carbon nanotubes in electric and magnetic fields," Phys. Rev. B **84**, 085452 (2011).
[8] E. A. Laird, F. Kuemmeth, G. A. Steele, K. Grove-Rasmussen, J. Nygård, K. Flensberg, and L. P. Kouwenhoven, "Quantum transport in carbon nanotubes," Rev. Mod. Phys. **87**, 703–764 (2015).
[9] Y. A. Kasumov, A. Shailos, I. I. Khodos, V. T. Volkov, V. I. Levashov, V. N. Matveev, S. Guéron, M. Kobylko, M. Kociak, H. Bouchiat, V. Agache, A. S. Rollier, L. Buchaillot, A. M. Bonnot, and A. Y. Kasumov, "CVD growth of carbon nanotubes at very low pressure of acetylene," Applied Physics A **88**, 687–691 (2007).
[10] E. D. Minot, Y. Yaish, V. Sazonova, and P. L. McEuen, "Determination of electron orbital magnetic moments in carbon nanotubes," Nature **428**, 536 (2004).
[11] F. Kuemmeth, S. Ilani, D. C. Ralph, and P. L. McEuen, "Coupling of spin and orbital motion of electrons in carbon nanotubes," Nature **452**, 448 (2008).
[12] S. H. Jhang, M. Marganska, Y. Skourski, D. Preusche, B. Witkamp, M. Grifoni, H. van der Zant, J. Wosnitza, and C. Strunk, "Spin-orbit interaction in chiral carbon nanotubes probed in pulsed magnetic fields," Phys. Rev. B **82**, 041404 (2010).
[13] T. S. Jespersen, K. Grove-Rasmussen, J. Paaske, K. Muraki, T. Fujisawa, J. Nygård, and K. Flensberg, "Gate-dependent spin-orbit coupling in multielectron carbon nanotubes," Nature Physics **7**, 348 (2011).
[14] T. S. Jespersen, K. Grove-Rasmussen, K. Flensberg, J. Paaske, K. Muraki, T. Fujisawa, and J. Nygård, "Gate-dependent orbital magnetic moments in carbon nanotubes," Phys. Rev. Lett. **107**, 186802 (2011).
[15] G. A. Steele, F. Pei, E. A. Laird, J. M. Jol, H. B. Meerwaldt, and L. P. Kouwenhoven, "Large spin-orbit coupling in carbon nanotubes," Nature Commun. **4**, 1573 (2013).
[16] This value is different from $L \sim 400\,\mathrm{nm}$ in Table **S-I** obtained from a fit of the $B_{\parallel}$ dependence of the lowest energy levels. Both values follow in one way or another from the assumption of sharp confinement, which is not realized in our device. With soft electrostatic confinement the most we can achieve is an estimate of an effective confinement length, which most likely lies between 240 and 400 nm.
[17] Ph. Lambin, V. Meunier, and A. Rubio, "Electronic structure of polychiral carbon nanotubes," Phys. Rev. B **62**, 5129–5135 (2000).
[18] F. Triozon, S. Roche, A. Rubio, and D. Mayou, "Electrical transport in carbon nanotubes: Role of disorder and helical symmetries," Phys. Rev. B **69**, 121410 (2004).
[19] M. Marganska, Sh. Wang, and M. Grifoni, "Electronic spectra of commensurate and incommensurate DWNTs in parallel magnetic field," New Journal of Physics **11**, 033031 (2009).
[20] S. Koller, M. Grifoni, M. Leijnse, and M. R. Wegewijs, "Density-operator approaches to transport through interacting quantum dots: Simplifications in fourth-order perturbation theory," Phys. Rev. B **82**, 235307 (2010).
[21] C. Sanderson and R. Curtin, "Armadillo: a template-based C++ library for linear algebra," The Journal of Open Source Software **1** (2016), 10.21105/joss.00026.
[22] K. Grove-Rasmussen, S. Grap, J. Paaske, K. Flensberg, S. Andergassen, V. Meden, H. I. Jørgensen, K. Muraki, and T. Fujisawa, "Magnetic-field dependence of tunnel couplings in carbon nanotube quantum dots," Phys. Rev. Lett. **108**, 176802 (2012).
[23] M. Niklas, S. Smirnov, D. Mantelli, M. Marganska, N.-V. Nguyen, W. Wernsdorfer, J.-P. Cleuziou, and M. Grifoni, "Blocking transport resonances via Kondo many-body entanglement in quantum dots," Nat. Commun. **7**, 12442 (2016).
